# Supplementary material for: Rethinking the Implementation Tricks and Monotonicity Constraint in Cooperative Multi-Agent Reinforcement Learning
Source: arXiv:2102.03479 source file (2023-06-08)
Supplement: Supplementary file 1 [file baseline.tex]

\subsection{Omitted Experimental Results}
%  We provide detailed experiment results to support our core statements.
We echo our experiments in Sec. \ref{section:QMIX with tricks}. Figure \ref{fig:baselines} shows that QMIX achieves excellent performance on all hard scenarios in SMAC and DEPP, and outperforms other algorithms.
Figure \ref{fig:baselines} also shows that QPLEX's policy collapses in the test of Super Hard $6h\_vs\_8z$ and $corridor$ \footnote{It may be that QPLEX feeds both actions and states into the mixing network in its implementation. The mixing network can predict true $Q_{tot}$ without correct $Q_i$, so that the $Q_i$ becomes useless.}. The win rates in Figure \ref{fig:baselines} are lower than in Table \ref{table:baselines} as we smoothed these curves.

\subsection{Omitted Experimental Results}
%  We provide detailed experiment results to support our core statements.
We echo our experiments in Sec. \ref{section:QMIX with tricks}. Figure \ref{fig:baselines} shows that QMIX achieves excellent performance on all hard scenarios in SMAC and DEPP, and outperforms other algorithms.
Figure \ref{fig:baselines} also shows that QPLEX's policy collapses in the test of Super Hard $6h\_vs\_8z$ and $corridor$ \footnote{It may be that QPLEX feeds both actions and states into the mixing network in its implementation. The mixing network can predict true $Q_{tot}$ without correct $Q_i$, so that the $Q_i$ becomes useless.}. The win rates in Figure \ref{fig:baselines} are lower than in Table \ref{table:baselines} as we smoothed these curves.
