# Supplementary material for: Rethinking the Implementation Tricks and Monotonicity Constraint in Cooperative Multi-Agent Reinforcement Learning
Source: arXiv:2102.03479 source file (2023-06-08)
Supplement: Supplementary file 2 [file cooperative.tex]

\section{Predator-Prey} \label{cpp}
In the vanilla Predator-Prey \cite{lowe2020multiagent}, three cooperating agents control three robot predators to chase a faster robot prey (the preys acts randomly) by controlling their velocities with actions [up, down, left, right, stop] within an area containing two large obstacles at random locations. The goal is to capture the prey with the fewest steps possible.

\textbf{Predator-Prey} By contrast, we use a variant of Predator-Prey from \cite{boehmer2020dcg} , which requires two predators to catch the prey at the same time to get a reward. Therefore, the variant requires effective agent coordination. However, \cite{boehmer2020dcg} added a penalty to the agents if only one predator catches the prey (not two predators at the same time), which makes the environments somewhat competitive. The penalty requires two predators capture the prey at the same time. If a diligent predator prefers to capture the prey and the other lazy one does not \footnote{Because of the random sampling in reinforcement learning, some samples with penalized rewards can cause certain agents to tend to be lazy.}, then they have conflicting interests. In our experiments, we remove the penalty to ensure that the environment is purely cooperative.

\textbf{Continuous Predator-Prey} We also use the Continuous Predator-Prey from \cite{peng2020facmac}. To obtain a hard cooperative environment, \cite{peng2020facmac} replaces the prey’s policy with a hard-coded heuristic that, at any time step, moves the prey to the sampled position with the largest distance to the closest predator. Therefore, the Continuous Predator-Prey is more difficult than the Predator-prey used by MADDPG \cite{lowe2020multiagent}.
