# Supplementary material for: Rethinking the Implementation Tricks and Monotonicity Constraint in Cooperative Multi-Agent Reinforcement Learning
Source: arXiv:2102.03479 source file (2023-06-08)
Supplement: Supplementary file 3 [file border_impact.tex]

\section{Broader Impact}
\label{appendix:Broader Impact}
Many complex real-world cooperative multi-robot problems can be simulated as CTDE multi-agent tasks. Specifically, decentralized agents can be applied to robot swarm control, vehicle coordination, and network routing. Applying MARL to these scenarios often requires a large number of samples to train the model, which implies high implementation costs, such as thousands of CPUs, power resources, and expensive robotic equipment, such as damaged drones or autonomous cars. Therefore, there is an urgent need to avoid any and all waste of such resources. In this work, the code-level optimizations and monotonicity constraint can help to improve the sample efficiency in some purely cooperative tasks, thereby reducing the wasting of resources.
